# Supplementary material for: Automated pulse discrimination of two freely-swimming weakly electric fish and analysis of their electrical behavior during a dominance contest
Source: arXiv:1607.00437 source file (2017-03-22)
Supplement: Supplementary file 1 [file supmat.pdf]

# Supplemental Material

## Automated pulse discrimination of two freely-swimming weakly electric fish and analysis of their electrical behavior during a dominance contest

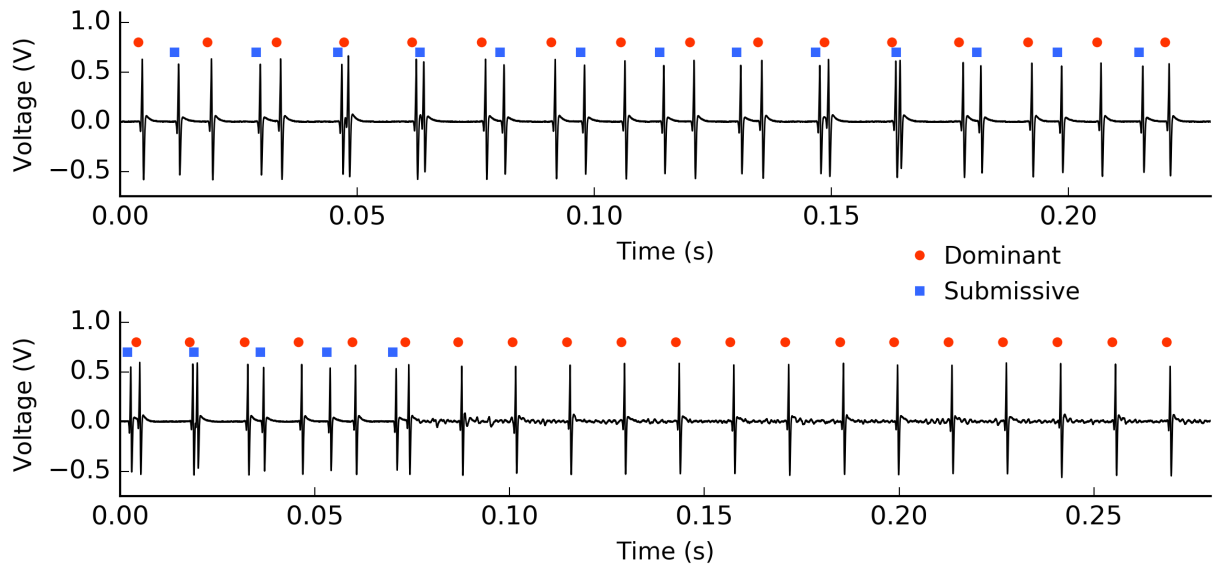

**Figure S1.** Pulse detection in a fine time scale using the automatic chirp detection. Each marker shows a pulse detected, with the color representing the emitter: either the dominant (red) or the submissive (blue) fish. **Top:** Example without chirp. **Bottom:** Example with chirp. This chirp starts after 0.07s, and no pulses from the submissive fish were detected. Only submissive fish presented chirps.

**Table S1.** Average and standard deviation of Inter Pulse Intervals (IPIs) for all fish dyads. We considered only of IPIs shorter than 40ms, so that offs are not included. When included, offs greatly increase the standard deviation of the IPIs. Results from three separate conditions are shown: each fish by itself (column Training), during the early contest ( $t < 430s$ ), and after the contest ( $t > 1000s$ ). Particularly, dyad 6 has a greater mean and standard deviation after 1000s. This is due to some periods on which the fish this dyad remained still, without interacting mechanically or electrically (See figure S3 for the IPI data). As this the only dyad who presented these differences and the only one recorded in 2016 (June 2016 for dyad 6 against September/October 2015 for dyads 1 – 5), its data is only included in this Supplemental Material and marked with a dagger.

| Dyad# | Status     | Training (ms)  | First 430 s (ms) | After 1000 s (ms) |
|-------|------------|----------------|------------------|-------------------|
| 1     | Dominant   | 15.8 $\pm$ 1.3 | 14.0 $\pm$ 1.0   | 13.8 $\pm$ 0.9    |
| 1     | Submissive | 15.1 $\pm$ 0.8 | 14.4 $\pm$ 0.9   | 16.6 $\pm$ 1.0    |
| 2     | Dominant   | 15.1 $\pm$ 0.8 | 14.4 $\pm$ 1.0   | 14.7 $\pm$ 0.8    |
| 2     | Submissive | 15.8 $\pm$ 1.3 | 16.0 $\pm$ 1.2   | 14.9 $\pm$ 1.0    |
| 3     | Dominant   | 15.3 $\pm$ 1.1 | 19.1 $\pm$ 1.9   | 18.5 $\pm$ 2.3    |
| 3     | Submissive | 19.8 $\pm$ 1.5 | 16.0 $\pm$ 0.9   | 16.4 $\pm$ 1.0    |
| 4     | Dominant   | 23.5 $\pm$ 5.3 | 20.8 $\pm$ 1.0   | 20.0 $\pm$ 0.9    |
| 4     | Submissive | 20.7 $\pm$ 1.6 | 22.9 $\pm$ 1.2   | 23.7 $\pm$ 1.5    |
| 5     | Dominant   | 16.8 $\pm$ 1.2 | 15.9 $\pm$ 2.0   | 16.2 $\pm$ 1.8    |
| 5     | Submissive | 17.3 $\pm$ 0.9 | 17.4 $\pm$ 2.0   | 19.3 $\pm$ 1.8    |
| 6†    | Dominant   | 27.6 $\pm$ 1.3 | 22.2 $\pm$ 1.7   | 26.3 $\pm$ 3.0    |
| 6†    | Submissive | 24.1 $\pm$ 2.3 | 24.9 $\pm$ 1.8   | 29.2 $\pm$ 2.6    |

**Table S2.** Comparing the statistics of Inter Pulse Intervals (IPI) between two phases: early dominance contest and post contest (referred in the table as  $t$  ( $1 \times 3$ )). We show paired Student's  $t$  statistics and its  $p$ -value. All submissive fish have significantly different IPIs when comparing different phases. For consistency, we also show the same statistical test applied to two regions randomly chosen from the post contest phase (in the table  $3 \times 3$ ). This is an indicative that our test is robust against pseudo-replication (see methodology section 2.8). The submissive fish from dyad 5 showed an outstanding number of offs and chirps, and the remaining data was not enough to compute its statistics.

| Dyad# | Status     | $t$ ( $1 \times 3$ ) | $p$ -value             | $t$ ( $3 \times 3$ ) | $p$ -value |
|-------|------------|----------------------|------------------------|----------------------|------------|
| 1     | Dominant   | 1.54                 | 0.15                   | 0.01                 | 0.99       |
| 1     | Submissive | -12.0                | $7.1 \times 10^{-12}$  | -0.15                | 0.88       |
| 2     | Dominant   | -3.57                | $1.30 \times 10^{-3}$  | -0.18                | 0.85       |
| 2     | Submissive | 11.09                | $1.03 \times 10^{-7}$  | -2.21                | 0.07       |
| 3     | Dominant   | 1.14                 | 0.26                   | -0.05                | 0.96       |
| 3     | Submissive | -2.6                 | 0.01                   | -0.83                | 0.41       |
| 4     | Dominant   | 4.05                 | $6.78 \times 10^{-4}$  | -0.32                | 0.75       |
| 4     | Submissive | -3.49                | $5.01 \times 10^{-3}$  | 0.59                 | 0.57       |
| 5     | Dominant   | -1.64                | 0.11                   | -1.49                | 0.15       |
| 5     | Submissive | –                    | –                      | –                    | –          |
| 6†    | Dominant   | -6.55                | $3.744 \times 10^{-6}$ | 0.45                 | 0.65       |
| 6†    | Submissive | -7.41                | $1.47 \times 10^{-6}$  | 1.06                 | 0.30       |

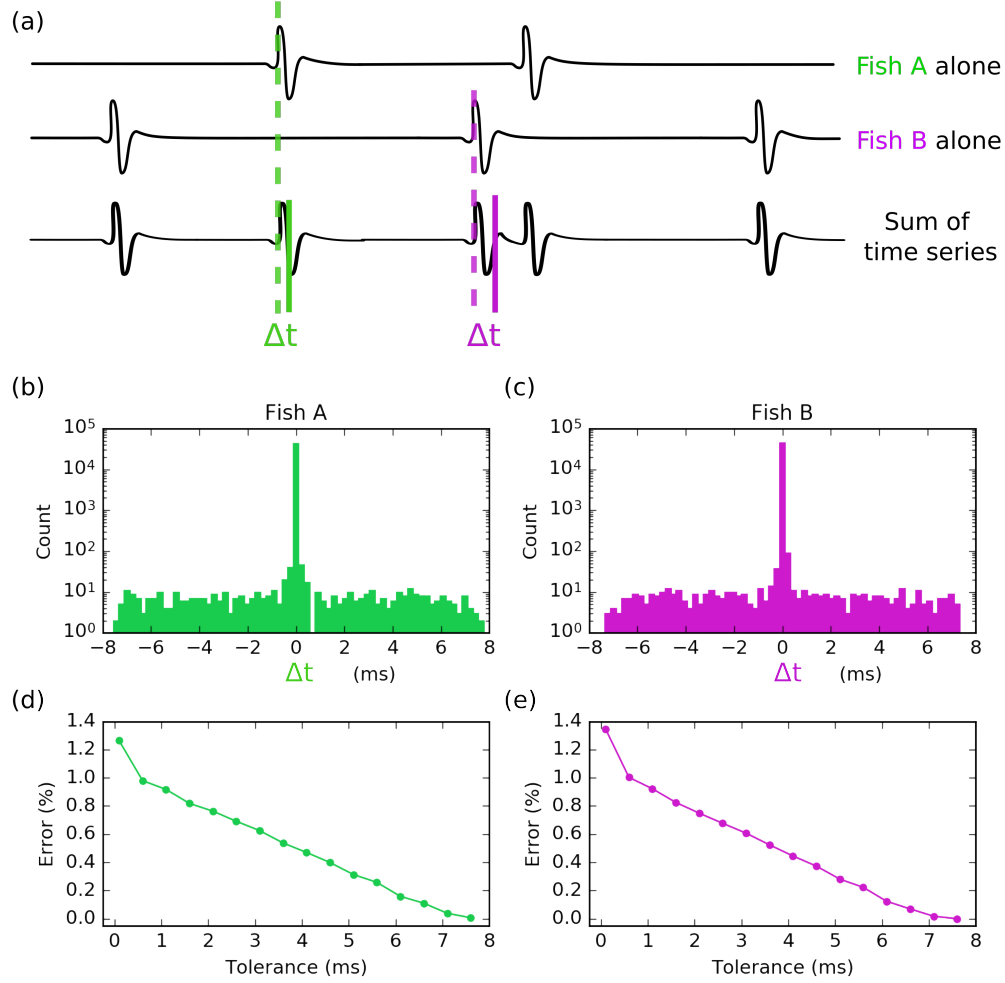

**Figure S2.** Temporal precision of the newly optimized algorithm using a synthetic time series (see text). **(a)** Detection delay is the time difference between the time stamp detected when using the time series of a single fish and the time stamp detected for that same pulse when the time series is summed with the pulses from another fish. Because both fish were never actually interacting, we refer to this summed time series as synthetic. **(b,c)** The algorithm detects pulses properly with minimal delay 5 orders of magnitude more frequently than detects with delays larger than 0.5ms. **(d,e)** Accuracy in classifying the correct pulse as function of the is below 1% for a tolerance of 0.5ms.

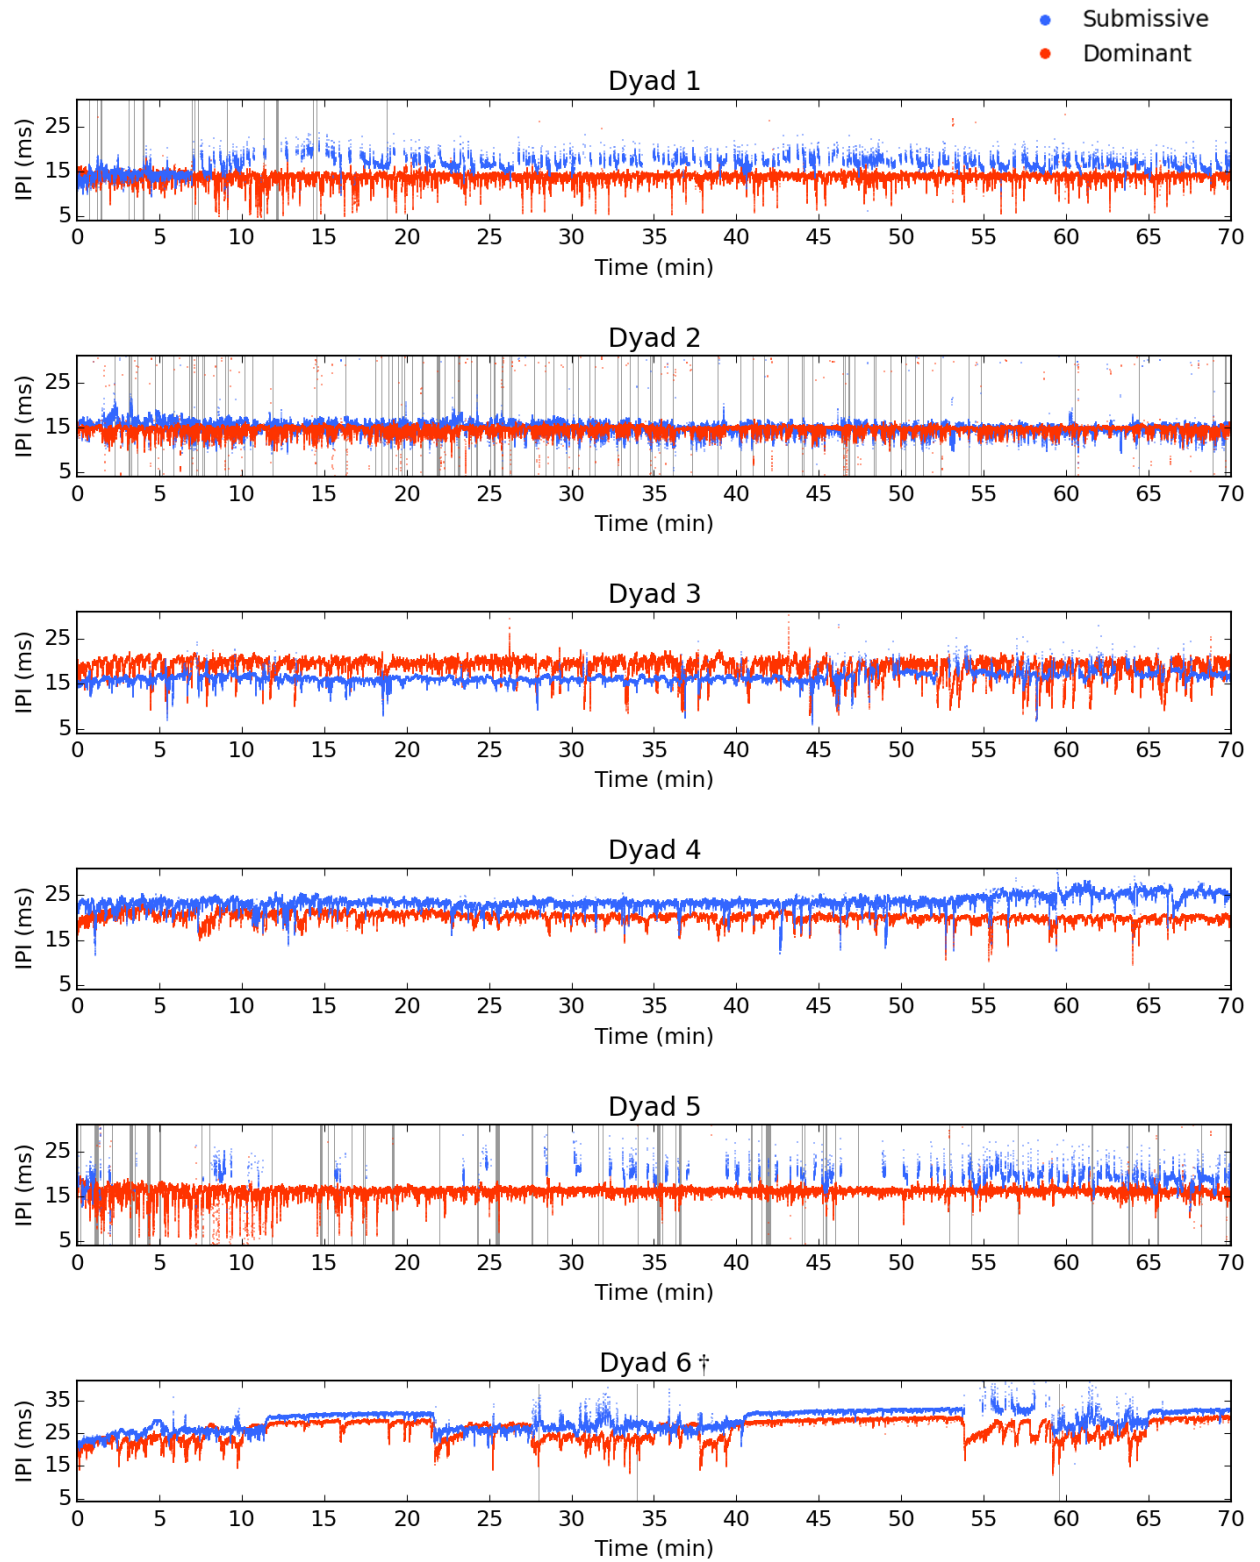

**Figure S3.** Time series of Inter Pulse Intervals (IPIs) for all five dyads considered. Long blank spaces are offs. Grey regions represent occurrence of chirps.

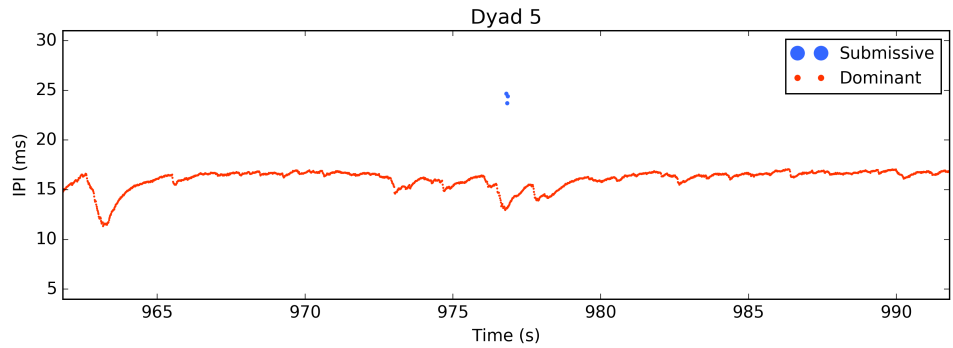

**Figure S4.** Example of pulses detected in between two periods of silence (off) of the submissive fish from dyad 5. These pulses from the submissive fish follow a period of 17 seconds of silence, and are followed by 78 seconds of another silent period. Due to the length of the recordings, isolated pulses between large silent periods become almost invisible to the naked eye (compare with Figure S3, bottom panel).

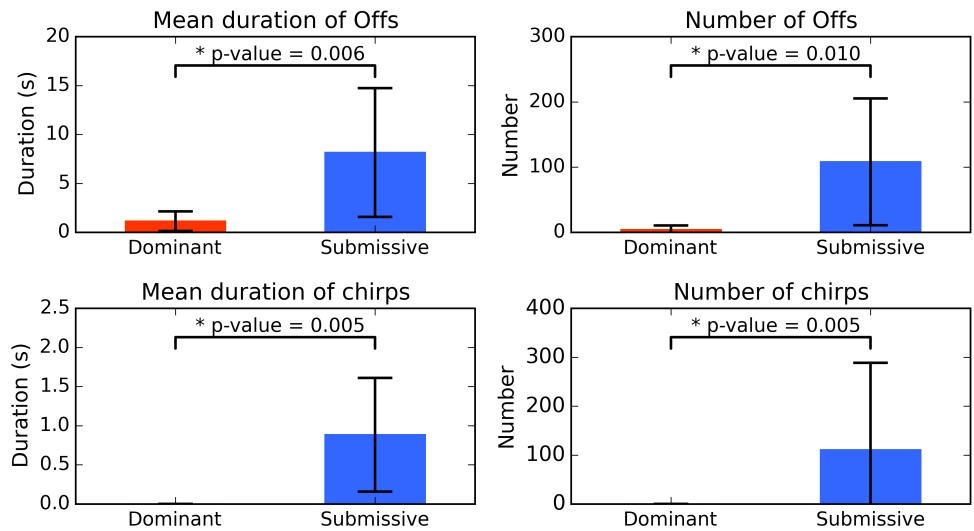

**Figure S5.** Dominant fish present significantly less offs and chirps than submissive fish. The number and duration of offs and chirps were treated separately for each fish to avoid pseudoreplication. The p-value was computed using the Mann-Whitney statistics. **Top-left:** The average duration of the offs observed in dominant fish was almost three times smaller than that of submissive fish. **Top-right:** The number of offs presented by submissive fish is remarkably larger than that of dominants. **Bottom-left:** The average duration of the chirps observed in submissive fish was about one second. Chirps were never observed in dominant fish. **Bottom-right:** On average, the submissive fish presented 100 chirps throughout the first hour of recording.

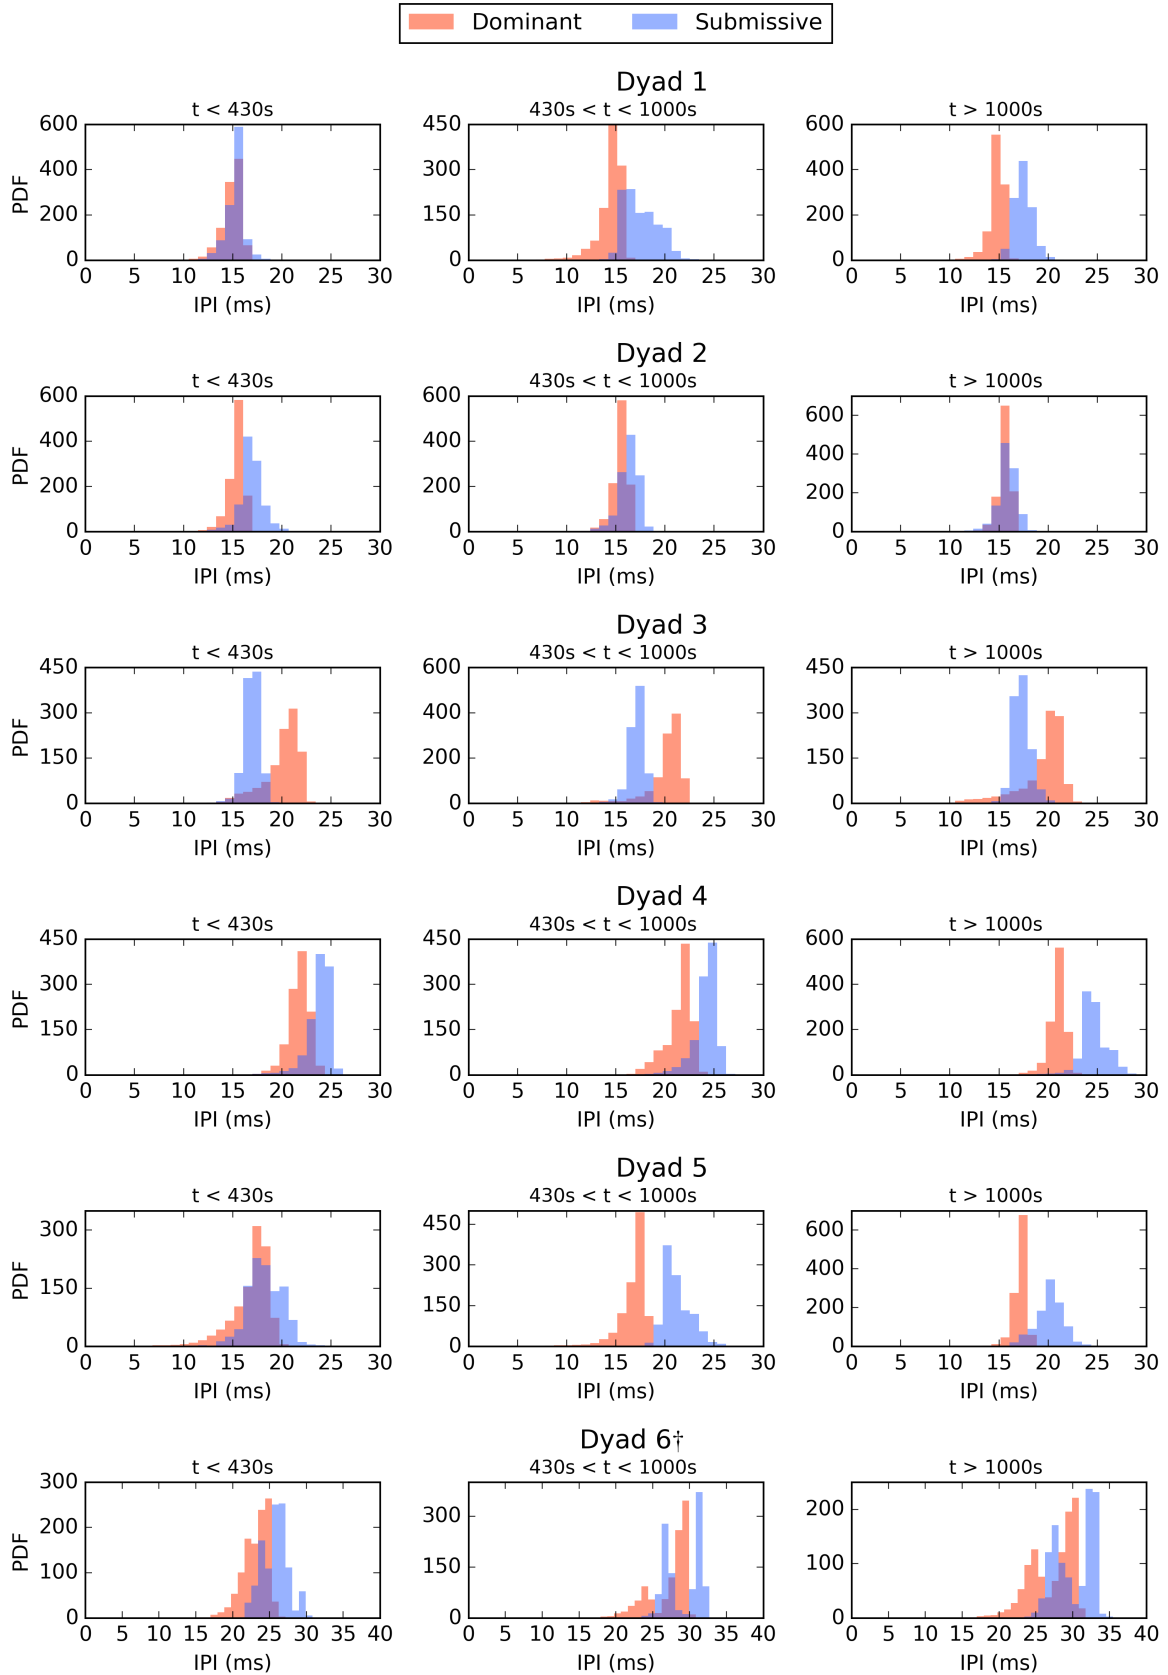

**Figure S6.** Distribution of Inter Pulse Intervals for all five dyads considered. Distributions are separated in three time phases: early dominance contest ( $t < 430s$ ), dominance contest ( $430s < t < 1000s$ ) and after contest ( $t > 1000s$ ).
